# Supplementary material for: Defect engineering-induced Seebeck coefficient and carrier concentration decoupling in CuI by noble gas ion implantation
Source: arXiv:2411.01015 source file (2024-11-01)
Supplement: Supplementary file 1 [file supplementaryMaterial.pdf]

# Supplementary material

## Defect engineering-induced Seebeck coefficient and carrier concentration decoupling in CuI by noble gas ion implantation

Martin Markwitz[1,2,3,*], Peter P. Murmu[2], Takao Mori[4,5], John V. Kennedy[2,3], Ben J. Ruck[1,3]

[1]School of Chemical and Physical Sciences, Victoria University of Wellington, PO Box 600, Wellington 6140, New Zealand

[2]National Isotope Centre, GNS Science, PO Box 30368, Lower Hutt 5010, New Zealand

[3]The MacDiarmid Institute for Advanced Materials and Nanotechnology, Victoria University of Wellington, PO Box 600, Wellington 6140, New Zealand

[4]International Center for Materials Nanoarchitectonics (WPI-MANA), National Institute for Materials Science (NIMS), 1-1 Namiki, Tsukuba, Ibaraki 305-0044, Japan

[5]Graduate School of Pure and Applied Science, University of Tsukuba, 1-1-1 Tennodai, Tsukuba, Ibaraki 305–8671, Japan

*** Corresponding author:** martin.markwitz@vuw.ac.nz

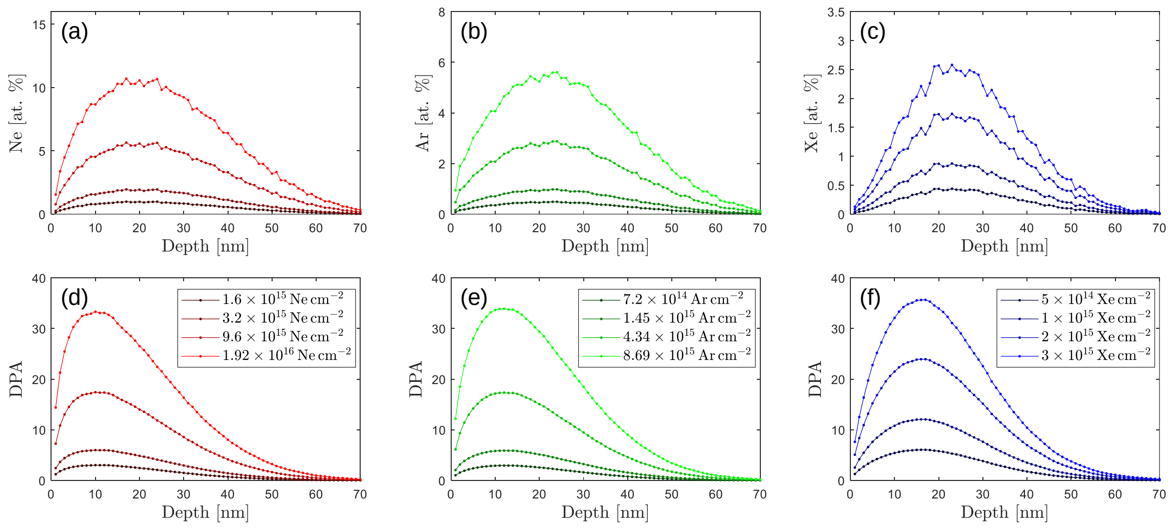


FIG. S1: (a) Neon 13 keV, (b) argon 27 keV, and (c) xenon 70 keV implantation concentration in CuI, and (d) neon, (e) argon, and (f) xenon DPA depth profiles calculated in in CuI with SRIM.

TABLE S1: Reprint of Table 1 from the manuscript, with the Label and film thickness columns added to clarify the sample identification in both the manuscript and supplementary information.

| Species | Energy [keV] | $F$ [ions cm$^{-2}$] | $D$ [disp. ion$^{-1}$] | DPA | Label | Film thickness [nm] |
|---|---|---|---|---|---|---|
| Ne | 13 | 0 | 200 | 0 | Ne-0 | 78±4 |
| Ne | 13 | $1.6 \times 10^{15}$ | 200 | 1.3 | Ne-1.3 | 71±4 |
| Ne | 13 | $3.2 \times 10^{15}$ | 200 | 2.5 | Ne-2.5 | 79±4 |
| Ne | 13 | $9.6 \times 10^{15}$ | 200 | 7.4 | Ne-7.4 | 58±3 |
| Ne | 13 | $1.92 \times 10^{16}$ | 200 | 14.1 | Ne-14.1 | 67±3 |
| Ar | 27 | 0 | 442 | 0 | Ar-0 | 70±4 |
| Ar | 27 | $7.2 \times 10^{14}$ | 442 | 1.3 | Ar-1.3 | 59±3 |
| Ar | 27 | $1.45 \times 10^{15}$ | 442 | 2.5 | Ar-2.5 | 52±3 |
| Ar | 27 | $4.34 \times 10^{15}$ | 442 | 7.5 | Ar-7.5 | 50±3 |
| Ar | 27 | $8.69 \times 10^{15}$ | 442 | 14.7 | Ar-14.7 | 45±2 |
| Xe | 70 | 0 | 1331 | 0 | Xe-0 | 58±3 |
| Xe | 70 | $5 \times 10^{14}$ | 1331 | 2.7 | Xe-2.7 | 61±3 |
| Xe | 70 | $1 \times 10^{15}$ | 1331 | 5.3 | Xe-5.3 | 63±3 |
| Xe | 70 | $2 \times 10^{15}$ | 1331 | 10.5 | Xe-10.5 | 42±2 |
| Xe | 70 | $3 \times 10^{15}$ | 1331 | 15.7 | Xe-15.7 | 53±3 |

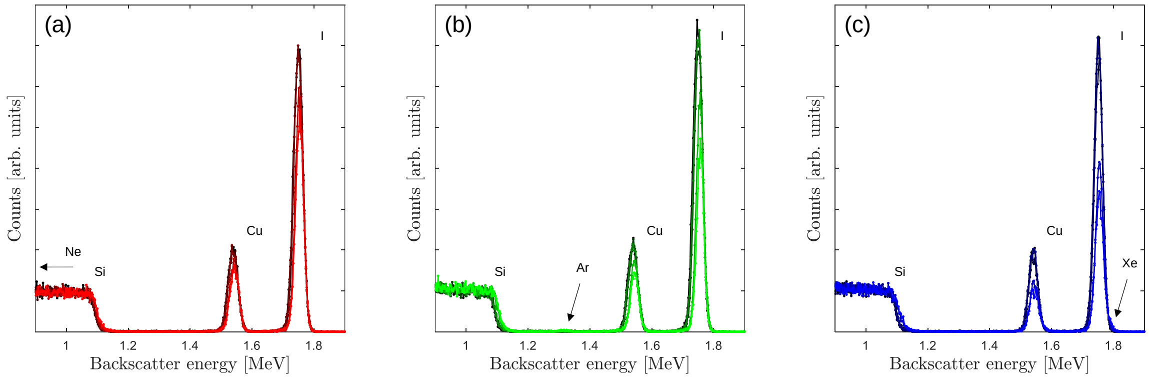


FIG. S2: RBS measurements of CuI films implanted with (a) neon, (b) argon, and (c) xenon. The same color sequence as FIG. S1 is applied.

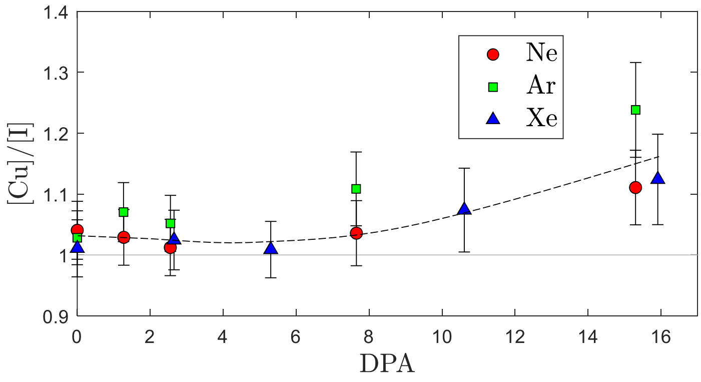


FIG. S3: [Cu]/[I] concentration ratios depending on the average DPA implantation species. Dashed line is used to guide the reader.

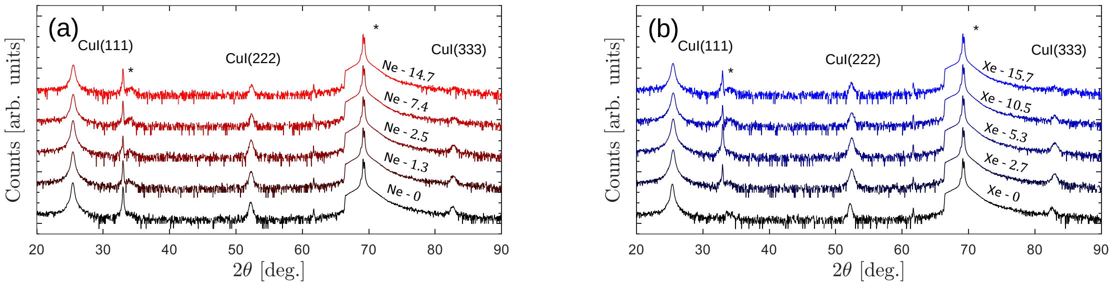


FIG. S4: Angle-symmetric X-ray diffractograms of samples implanted with (a) neon and (b) xenon. XRD patterns are vertically offset for visual clarity.

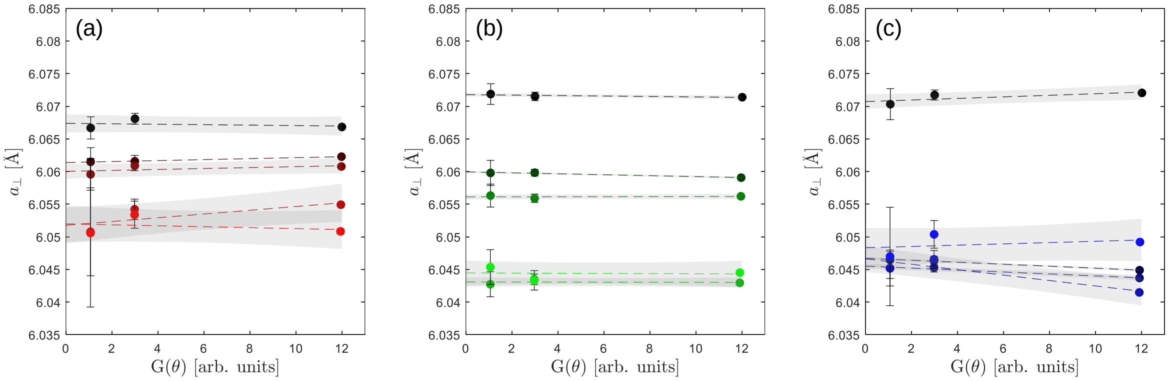


FIG. S5: Goniometer error function fits applied to calculated peak positions of CuI films implanted with (a) neon, (b) argon, and (c) xenon. The same color sequence as FIG. S1 is applied.
